# Supplementary material for: A New Algorithm for Decremental Single-Source Shortest Paths with Applications to Vertex-Capacitated Flow and Cut Problems
Source: arXiv:1905.11512 source file (2019-05-27)
Supplement: Supplementary file 1 [file appendix-ES-trees.tex]

%----------------------------------
%----------------------------------
\subsection{ES-Trees}\label{subsec: ES-trees}
%----------------------------------
%----------------------------------
%----------------------------------
Even-Shiloach tree (\EST) is a deterministic data structure for decremental single-source shortest-path. Given a graph $G=(V,E)$ with integral lengths $\ell(e)\geq 1$ on its edges $e\in E$, a source $s$, and a distance bound $D\geq 1$, the data structure, denoted by $\EST(G,s,D)$  maintains a shortest-path tree $T$ rooted at $s$ up to distance $D$ (that is, a vertex $v\in T$ iff $\dist_G(s,v)\leq D$, and, for every vertex $v$ with $\dist(s,v)\leq D$, the distance $\dist(s,v)$). The data structure supports two operations:

\begin{itemize}
\item Edge Deletion, denoted by $\ESTDEL(G,e)$: delete an edge $e\in E(G)$ from graph $G$; and
%\item Vertex Insertion, denoted by $\ESTVIN(G,v)$: insert  a new isolated vertex $v$ into $G$; and
\item Edge Insertion, denoted by $\ESTIN(G,e)$: insert an eligible edge $e$ into $G$; edge $e$ is eligible for insertion, if its insertion does not decrease distances between any pair of vertices.
\end{itemize}

%We denote the corresponding data structure, that we describe below, by $\EST(G,s,D)$. %When the distance bound $D$ is unbounded (that is, $D=nW$, where $W=\max_{e\in E}\set{w(e)}$), then we denote the data structure by $\EST(G,s)$.
The total running time of the algorithm, including the initialization and updates, is $O(mD\log m)+O(n)$, where $m$ is the total number of edges that are ever present in the graph, and $n=|V(G)|$.

Throughout the algorithm, we maintain a shortest-path tree $T$ from $s$, up to distance $D$. The algorithm is partitioned into phases, where in every phase one of the operations $\ESTDEL$ or $\ESTIN$ is performed, and the data structure is updated -- we call the latter step an update procedure. 

The algorithm uses a number of heaps, where the number of elements in each heap is bounded by $m$. We perform basic operations on heaps, that include: returning an element with smallest key; inserting an element; and deleting an element. Each such operation can be executed in $O(\log m)$ time. We let $\eta=c\log m$ for large enough constant $c$, so that in time $\eta$ we can execute a constant number (say $20$) of basic heap operations. 

\paragraph{The Data Structure.}
Throughout the algorithm, we maintain a shortest-path tree $T$ from $s$, up to distance $D$. We also maintain, for every vertex $v\in V$, a label $\delta(v)$. The algorithm guarantees that for all $v\in V$, if $\dist(s,v)\leq D$, then $\delta(v)=\dist(s,v)$, except during an update procedure for $\ESTDEL$, when it only guarantees that $\delta(v)\leq \dist(s,v)$. If $\dist(s,v)>D$, then the algorithm guarantees that $\delta(v)=\infty$ and $v\not \in T$.

For every vertex $v\in V$, we maintain a heap $H(v)$, that stores, for every neighbor $u$ of $v$ in $G$, the vertex $u$ with the key $\ell(u,v)+\delta(u)$. Vertex $v$ has pointers to all its copies in the heaps of all its neighbors.

\paragraph{Initialization.}
To initialize, we build a shortest-path tree $T$ from $s$, using the algorithm of Thorup~\cite{linear-sssp} in $O(m)$ time, and compute the labels $\delta(v)$ for all vertices $v\in V$. We also initialize the heaps $H(v)$ for every vertex $v$. In order to do so, for every vertex $v\in V$, we start with an empty heap $H_v$, and then, for every neighbor $u$ of $v$, we insert the vertex $u$ into $H_v$ with the key $\delta(u)+\ell(u,v)$, adding pointers between $u$ and its copy in $H_v$. For vertices $v$ that do not belong to $T$ or have $\dist(s,v)>D$, we set $\delta(v)=\infty$.  All this can be done in time $O(m+n)$. 

\paragraph{Edge Insertion.}
In the $\ESTIN(G,e)$ operation, we are given an edge $e=(u,v)$ that does not currently belong to $G$, such that the insertion of $e$ does not decrease the distances between any pair of vertices, and we need to insert the edge $e$ into $G$. 
Notice that the tree $T$ remains a valid shortest-path tree in the new graph, and the labels $\delta(x)$ for vertices $x\in V$ remain correct. We update the heaps $H_u$ and $H_v$ by inserting $v$ into $H_u$ with key $\delta(v)+\ell(u,v)$, and $u$ into $H_v$, with key $\delta(u)+\ell(u,v)$, using two basic heap operations, in time $O(\log n)$. Overall, the total update time of the algorithm due to $\ESTIN$ operations is $O(m\log n)$.

\paragraph{Edge Deletion.}
We now describe an update procedure for $\ESTDEL$ operation.

Over the course of the update procedure, we inspect a number of vertices. An inspection of a vertex $v$ consists of a constant number of basic heap operations, and its running time is bounded by $\eta$.
The key invariant of the algorithm, that allows us to bound its total running time, is that we only inspect a vertex $v$ in one of the following three cases:

\begin{enumerate}
\item If an edge incident to $v$ is deleted -- there can be at most $2m$ such inspections over the course of the algorithm;

\item If $\delta(v)$ increases -- this can happen at most $D$ times for each vertex $v$, so the total number of such inspections, over the course of the algorithm,  is bounded by $nD$; %Each such inspection is charged to the vertex $v$; 
and

\item If $\delta(u)$ increases for one of the neighbors of $u$. For every vertex $v$, for each increase of $\delta(v)$, we may need to inspect up to $d(v)$ vertices -- the neighbors of $v$ in $G$. As $\delta(v)$ may grow at most $D$ times, the total number of such inspections, over the course of the algorithm, is bounded by $\sum_{v\in V}D\cdot d(v)=O(mD)$. %If we inspect $u$ because $\delta(v)$ increases for one of its neighbors $v$, we charge this inspection to the edge $(u,v)$, so every edge is charged at most $2D$ times.
\end{enumerate}

Clearly, if the above invariant holds throughout the algorithm, the total update time of the algorithm due to $\ESTDEL$ operations is $O(mD\eta)=O(mD\log n)$.

\paragraph{Update Procedure.}
Consider a phase when some edge $e=(u,v)$ is deleted from the graph. If this edge does not belong to the current tree $T$, then the distances $\dist(s,x)$ for vertices $x\in V$ do not change, and we terminate the update procedure. Therefore, we assume from now on that $e$ is an edge of the tree $T$, and we assume w.l.o.g. that $u$ is the parent of $v$ in $T$. Let $T_v$ be the sub-tree of $T$ rooted at $v$. Note that $\dist(s,v)$ may change as the result of deleting $e$, and this change may propagate to vertices of $T_v$.

Throughout the update procedure, we will maintain a heap $H$, containing vertices of $T_v$ that we need to inspect. The key stored with each vertex $x$ in $H$ is the current value $\delta(x)$. As the update procedure progresses, $\delta(x)$ may grow. 
At the beginning, $H$ contains a single vertex -- the vertex $v$.
Over the course of the algorithm, every vertex $x$ of $T_v$ is in one of the following four states:

\begin{itemize}
\item {\bf Untouched:} we have never inspected $x$, and it is not currently attached to the tree $T$. If $x$ is untouched, then it does not belong to $H$, and we do not know whether $\dist(s,x)$ has increased. The value $\delta(x)$ did not change during the current update procedure yet.
\item {\bf Settled:} we attached $x$ to the tree, and its current value $\delta(x)=\dist(s,x)$ in the new graph. A settled vertex does not belong to the heap $H$.
\item {\bf Suspicious:} We have added $x$ to the heap $H$ but we did not inspect it yet, and $\delta(x)$ has not changed yet. However, if $y$ is the parent of $x$ in $T_v$, then $\delta(y)$ has increased. A suspicious vertex is not attached to the tree $T$; and
\item {\bf Changed:} we have increased $\delta(x)$ in the current iteration, but we do not yet know the value of $\dist(s,x)$. All changed vertices belong to $H$, and a changed vertex is not attached to the tree. When a vertex becomes changed for the first time, all its children are added to $H$ as suspicious vertices.
\end{itemize}

%Intuitively, if we consider the tree $T_v$ during any point of the update procedure, then the vertices that were added to $H$ over the course of the update procedure so far (including the vertices that later became settled) induce a connected sub-tree of $T_v$ that includes $v$. Let us denote this sub-tree by $T'$. The leaves of $T'$ are the vertices $x$ for which $\delta(x)$ has not yet changed -- these are the vertices that were added to $H$ as suspicious vertices but have not yet become changed vertices; some of them may have become settled. The inner vertices of $T'$ are those vertices $x$ for which $\delta(x)$ has increased over the course of the update procedure -- these are the vertices that became changed, and some of them may have become settled. As we will see, if any vertex $x$ is untouched, then it has some ancestor that currently belongs to the heap $H$ as a suspicious vertex.

We ensure that throughout the update procedure, the following invariants hold:

\begin{properties}{I}
\item For all $x\in T_v$, $\delta(x)\leq \dist(s,x)$. Moreover, if $x$ is a settled vertex, then $\delta(x)=\dist(s,x)$; \label{inv: delta}

\item For all $x\in T_v$, if $x$ is or was a changed vertex, then all its children were added to $H$ when $x$ became changed; and \label{inv: changed children}

\item If $x\in T_v$ is an untouched vertex, then some ancestor of $x$ is currently a suspicious vertex. \label{suspicious: ancestor}
\end{properties}

Assuming that the above invariants hold, we obtain the following observation.

\begin{observation}\label{obs: smallest key}
Let $x$ be a vertex in $H$, with minimum $\delta(x)$, and let $y\in H_x$ be the vertex minimizing $\delta(y)+\ell(x,y)$. Assume further that $ \delta(y)+\ell(x,y)\leq \delta(x)$. Then either $y\in T\setminus T_v$, or $y$ is settled; in other words, $y$ is currently attached to $T$. Moreover, $\delta(x)=\delta(y)+\ell(x,y)$.
\end{observation}
\begin{proof}
Assume that $y$ is not currently attached to $T$. Then either $y\in H$, or $y$ is untouched. If $y\in H$, then $\delta(y)\geq \delta(x)$ from the choice of $x$, and, since $\ell(x,y)\geq 1$, it is impossible that $\delta(y)+\ell(x,y)\leq \delta(x)$. Therefore, $y$ is untouched. But then $y$ has an ancestor $y'$ that is a suspicious vertex. Therefore, $\delta(y')$ did not grow during the current update operation yet, and so $\delta(y')<\delta(y)$ still holds. As $y'$ is a suspicious vertex, $y'\in H$. From the choice of $x$, $\delta(x)\leq \delta(y')<\delta(y)$, a contradiction. Therefore, $y$ is currently attached to the tree $T$.

From Invariant~\ref{inv: delta}, $\delta(y)=\dist(s,y)$, and $\delta(x)\leq \dist(s,x)$. Since there is a path from $x$ to $s$ of length $\delta(y)+\ell(x,y)\leq \delta(x)$, it follows that $\delta(x)=\delta(y)+\ell(x,y)$.
\end{proof}

We are now ready to describe the update procedure. At the beginning, the heap $H$ only contains the vertex $v$, which is a suspicious vertex. All other vertices of $T_v$ are untouched. Observe that all invariants hold. We now describe an iteration of the update procedure, assuming that all invariants hold at the beginning of the iteration.

Let $x\in H$ be the vertex with the smallest key $\delta(x)$. If $\delta(x)>D$, then we terminate the update procedure -- every vertex $y$ that is not currently attached to the tree $T$ has $\dist(s,y)>D$. Each such vertex either belongs to $H$, or is a descendant, in the original tree $T_v$, of a vertex in $H$. For each such vertex $y$, we set $\delta(y)=\infty$, and we delete $y$ from the heaps of its neighbors. Notice that this operation is performed at most once per vertex over the course of the algorithm, and contributes at most $O(m\eta)$ to the total running time.

Therefore, we assume that $\delta(x)\leq D$. Let $y\in H_x$ be the vertex minimizing $\delta(y)+\ell(x,y)$. We now consider two cases. The first case happens when  $\delta(y)+\ell(x,y)\leq \delta(x)$. Then, from Observation~\ref{obs: smallest key}, $y$ is currently attached to the tree $T$, and $\delta(y)+\ell(x,y)= \delta(x)$. We attach $x$ to the tree $T$ as a child of $y$, and $x$ becomes a settled vertex. (Note that if $x$ was not yet inspected in this update procedure, that is, we never changed $\delta(x)$, then all its descendants are untouched, and they get attached to the tree together with $x$. In that case, all descendants of $x$ become settled vertices. Otherwise, $x$ was a changed vertex at the beginning of this iteration, and so all its children were added to the heap $H$. We do not reattach any of its descendants to the tree then.) It is immediate to verify that all invariants continue to hold.

Otherwise, $\delta(y)+\ell(x,y)> \delta(x)$. Then from Invariant~\ref{inv: delta}, we know that the current estimate of $\delta(x)$ is too small. We then increase $\delta(x)$ by $1$ and return $x$ to $H$. If this is the first time that $\delta(x)$ is increased in the current iteration, then it becomes a changed vertex, and all its children in the tree $T_v$ become suspicious and are added to the heap $H$. In any case, we update the key of $x$ in the heaps $H_z$ for all neighbors $z$ of $x$.  It is immediate to verify that all invariants continue to hold.

We now analyze the running time of the update procedure. Consider an iteration when a vertex $x$ is processed. We need to perform two basic heap operations: delete $x$ from $H$ and find the smallest element of $H_x$. We now consider two cases. The first case happens when  $\delta(x)$ increases in the current iteration. Then we need to update all the heaps $H_z$ of every neighbor $z$ of $x$, where each update involves a single basic heap operation (increase the key associated with $x$). Additionally, for every child vertex $z'$ of $x$ that becomes suspicious but never becomes changed, we will later inspect $z$, and charge the processing time of this inspection to $x$. 

Assume now that $\delta(x)$ does not increase, that is, $x$ becomes a settled vertex. If $x$ was a changed vertex, then we charge this inspection of $x$ to $x$ itself. If $x$ was a suspicious vertex, then this inspection (that only involves two basic heap operations) is charged to its (changed) parent in the tree (in the case where $x=v$, we charge the deleted edge $(u,v)$). We do not need to explicitly update the status of its descendants to ``settled'': the algorithm naturally ensures that these vertices are never added to $H$.

Overall, the inspection of a vertex requires a constant number of calls to basic heap operations, and we assume that the running time of such an inspection is at most $\eta$. A vertex $x$ is inspected either when it is incident to an edge that was deleted, or if $\delta(x)$ grows, or if there is some neighbor $z$ of $x$, such that $\delta(z)$ grows. As discussed above, the total update time of the algorithm due to the \ESTDEL operations is then bounded by $O(mD\eta)=O(mD\log n)$.
%So far we have assumed that only $\ESTDEL$ operations are allowed. Next, we extend this algorithm to handle $\ESTIN$ and $\ESTVIN$ operation.

We conclude that the total running time of the algorithm, including initialization and update time due to $\ESTDEL$ and $\ESTIN$ operations is bounded by $O(mD\log m)+O(n)$.
