# Supplementary material for: A New Algorithm for Decremental Single-Source Shortest Paths with Applications to Vertex-Capacitated Flow and Cut Problems
Source: arXiv:1905.11512 source file (2019-05-27)
Supplement: Supplementary file 2 [file appendix-Bernstein-old.tex]

%--------------------------------------------------------
%--------------------------------------------------------
\subsection{Proof of Theorem~\ref{thm: WSES}}
%---------------------------------------------------------
%---------------------------------------------------------
%--------------------------------------------------------
%--------------------------------------------------------
 Recall that the original ES algorithm stored, together with every vertex $v$, a value $\delta(v)$, which was the distance from $s$ to $v$. We will no longer ensure that $\delta(v)=\dist_G(s,v)$, but rather that $\dist_G(s,v)\leq \delta(v)\leq (1+\eps)\dist_G(s,v)$.
 Recall that in the ES-procedure, whenever $\delta(v)$ increases, we immediately update the copies of $v$ in the heaps $H_u$ of its neighbors to reflect this change. In the modified algorithm, every neighbor $u$ of $v$ will keep a copy $\delta_u(v)$ of the value $\delta(v)$, that is not necessarily up to date, and will only be updated when $\delta(v)$ increases significantly relatively to $\ell(u,v)$.
We will use the following definition.


\begin{definition}
Given an edge $e$ and an integer $x$, $\round_e(x)$ is the smallest integer $y>x$ that is an integral multiple of $\eps \ell(e)$.
\end{definition}

Intuitively, $\delta_v(u)$ is only updated once the value of $\delta(u)$ increases by $\round_e(?)$.


We now give a quick overview of edge insertion, which becomes somewhat more complicated. Suppose we would like to insert an edge $e=(u,v)$, where $\dist_G(s,u)=1000$, $\dist_G(s,v)=1000$, and $\ell(e)=1$. It is easy to verify that edge $e$ is eligible for insertion, as for all $x\in V(G)$, $\dist_G(s,x)$ does not decrease. But because we maintain approximate distances from $s$, we may have $\delta(u)=1000$ and $\delta(v)=1000(1+\eps)$. We need to insert a copy $\delta_v(u)$ of $u$ into the heap of $v$ and decrease $\delta(v)$ accordingly, but, since the algorithm analysis depends on the fact that the values $\delta(v)$ never increase, it is not clear how to do so.

The following definition will be used to handle this difficulty.

\begin{definition}
Let $v\in V(G)$, and let $e=(u,v)$ be an edge incident to $v$ that was inserted into $G$, so in particular $e$ is an eligible edge. We say that $(e,v)$ is a \emph{problematic pair} iff $\delta(u)+\ell(u,v)< \delta(v)$ at the time when $e$ was inserted. In such a case, we set $\delta_v(u)=\delta(v)-\ell(u,v)$. The value $\delta_v(u)$ is not updated by the algorithm, until $\delta_u$ becomes greater than $\delta_v(u)$, at which point $(e,v)$ stop being problematic, and $\delta_v(u)$ is updated as usual.
\end{definition}

 The intuitive idea is that the original value $\delta(v)$ was a $(1+\eps)$-approximation on $\dist_G(s,v)$, and, as long as $\delta(u)\leq \delta(v)-\ell(u,v)$, we know that $\dist_G(s,v)\leq \delta(v)$. Since the distances from $s$ never decrease, $\delta(v)$ remains a $(1+\eps)$-approximation to $\dist_G(s,v)$.

Throughout the algorithm, we ensure that between updates, the values $\delta(v)$ for $v\in V(G)$ will have the following two properties:


\iffalse
\begin{properties}{I}
\item If $v=s$, then $\delta(v)=0$. Otherwise, if $p$ is the parent of $v$ in the current tree $T$, then $\delta(v)\geq \delta(p)+\ell(p,v)$; and \label{inv1: father}
\item For every neighbor $u$ of $v$, $\delta(v)\leq \delta(u)+(1+\eps)\ell(u,v)$. \label{inv1: neighbor}
\end{properties}
\fi



\begin{properties}{J}
\item if $v=s$, then $\delta(v)=0$. Otherwise, if $p$ is the parent of $v$ in the current tree $T$, then $\delta(v)\geq \delta(p)+\ell(p,v)$; and \label{inv12: father}

\item for every vertex $v\in V(G)$ and edge $e=(u,v)$ incident to it, if $(e,v)$ is not a problematic pair, then $\delta(v)\leq \delta(u)+(1+\eps)\ell(u,v)$. \label{inv12: neighbor}
\end{properties}



\begin{claim}\label{claim: approx}
Assume that invariants (\ref{inv12: father}) and (\ref{inv12: neighbor}) hold throughout the algorithm. Then throughout the algorithm, for each $v\in T$, $\dist_G(s,v)\leq \delta(v)\leq (1+\eps)\dist_G(s,v)$.
\end{claim}
\begin{proof}
To see that $\delta(v)\geq \dist_G(s,v)$, we simply follow the path in the tree $T$ from $v$ to $s$. From the first invariant, $\delta(v)$ is at least the sum of weights of edges along this path, which is at least $\dist_G(s,v)$. We now turn to prove that $\delta(v)\leq (1+\eps)\dist_G(s,v)$.

The proof is by induction on time and the length of the shortest path from $s$ to $v$. 
When the algorithm starts, for every vertex $v$, $\delta(v)=\dist_G(s,v)$. We now consider the state of the algorithm after some iteration $j$, and consider the shortest $s-v$ path.
If this path contains no edges, then $\delta(s)=0$, and we are done.  Assume now that the shortest $s$-$v$ path has $i>0$ edges. Let $u$ be the penultimate vertex on this path, and let $e=(u,v)$ be the corresponding edge.
Then $\dist_G(s,v)=\dist_G(s,u)+\ell(u,v)$.
Assume first that $(e,v)$ is not a problematic pair.
From the induction hypothesis, $\delta(u)\leq (1+\eps)\dist_G(s,u)$. From the second invariant, $\delta(v)\leq \delta(u)+(1+\eps)\ell(u,v)\leq (1+\eps)\dist_G(s,u)+(1+\eps)\ell(u,v)=(1+\eps)\dist_G(s,v)$.

Finally, assume that $(e,v)$ is a problematic pair. 
 Then, by the induction hypothesis, when $e$ was added to the graph, $\delta(v)\leq (1+\eps)\dist_G(s,v)$ held. As long as $(e,v)$ remains a problematic pair, $\delta(v)$ does not grow, but $\dist_G(s,v)$ may increase. Therefore, $\delta(v)\leq (1+\eps)\dist_G(s,v)$ continues to hold. 
 \end{proof}





%We first show that, if the above invariants are maintained, then we indeed maintain approximate shortest paths from $s$.
%\begin{claim}\label{claim: approx}
%Assume that the values $\delta(v)$ for $v\in T$ obey the above invariants. Then for each $v\in T$, $\dist_G(s,v)\leq \delta(v)\leq (1+\eps)\dist_G(s,v)$.
%\end{claim}
%\begin{proof}
%To see that $\delta(v)\geq \dist_G(s,v)$, we simply follow the path in the tree $T$ from $v$ to $s$. From the first invariant, $\delta(v)$ is at least the sum of weights of edges along this path, which is at least $\dist_G(s,v)$. We now turn to prove that $\delta(v)\leq (1+\eps)\dist_G(s,v)$.

%The proof is by induction on the number of edges in the shortest path from $s$ to $v$. If the shortest path contains just one edge $e$, then 
%$\delta(v)\leq \delta(s)+(1+\eps)\ell(e)$. Assume now that the shortest $s$-$v$ path has $i>1$ edges, and let $u$ be the penultimate vertex on this path. Then $\dist_G(s,v)=\dist_G(s,u)+\ell(u,v)$. From the induction hypothesis, $\delta(u)\leq (1+\eps)\dist_G(s,u)$. From the second invariant, $\delta(v)\leq \delta(u)+(1+\eps)\ell(u,v)\leq (1+\eps)\dist_G(s,u)+(1+\eps)\ell(u,v)=(1+\eps)\dist_G(s,v)$.
%\end{proof}


%Recall that in the ES-procedure, whenever $\delta(v)$ increases, we immediately update the copies of $v$ in the heaps $H_u$ of its neighbors to reflect this change. In the modified algorithm, every neighbor $u$ of $v$ will keep a copy $\delta_u(v)$ of the value $\delta(v)$, that is not necessarily up to date. 

We replace the invariants~(\ref{inv12: father}) and (\ref{inv12: neighbor}) with the following two approximation invariants, that hold for every vertex $v$ throughout the algorithm:

\begin{properties}{A}
\item If $v=s$, then $\delta(v)=0$. Otherwise, let $u$ be the parent of $v$ in the tree. Then $\delta(v)=\delta_v(u)+\ell(u,v)$. (that is, we use the approximate local estimate on $\delta(u)$ in order to establish $\delta(v)$). Moreover, $u$ is the neighbor of $v$ with minimum $\delta_v(u)+\ell(u,v)$.
\label{inv2: approx father}


\item If $e=(u,v)$ is an edge incident to $v$, then $\delta_v(u)\geq \delta(u)$. Moreover, if $(e,v)$ is not a problematic pair, then $\delta_v(u)\leq \round_e(\delta(u))$.\label{inv2: approx neighbor}
\end{properties}

\begin{observation}
If Invariants~(\ref{inv2: approx father}) and~(\ref{inv2: approx neighbor}) hold throughout the algorithm, so do Invariants~(\ref{inv12: father}) and (\ref{inv12: neighbor}).
\end{observation}

\begin{proof}
In order to establish Invariant~(\ref{inv12: father}), observe that, if $s=v$, then invariant~(\ref{inv2: approx father}) guarantees that $\delta(v)=0$. Otherwise, let $u$ be the parent of $v$ in the tree. Then, from Invariant~(\ref{inv2: approx father}), $\delta(v)=\delta_v(u)+\ell(u,v)$, and, from Invariant~(\ref{inv2: approx neighbor}), $\delta_v(u)\geq \delta(u)$, so $\delta(v)\geq \delta(u)+\ell(u,v)$.

In order to establish Invariant~(\ref{inv12: neighbor}), let $e$ be an edge incident to $v$, such that $(e,v)$ is not a problematic pair. Then, from Invariants ~(\ref{inv2: approx father}) and (\ref{inv2: approx neighbor}):

\[\delta(v)\leq \delta_v(u)+\ell(e)\leq \round_e(\delta(u))+\ell(e)\leq \delta(u)+(1+\eps)\ell(e).\]

\end{proof}

Therefore, it is now enough to maintain Invariants~\ref{inv2: approx father} and \ref{inv2: approx neighbor}.


In order to obtain the improved running time, we implement the following changes:

\begin{itemize}
\item Whenever $\delta(v)$ increases, we can inspect it, and charge the vertex for the inspection. However, we do not immediately inspect its neighbors. The number of such inspections is bounded by $nD$.

\item Let $e=(u,v)$ be an edge. We charge this edge (by inspecting both its endpoints) only if $\round_e(\delta(u))$ increases or $\round_e(\delta(v))$ increases. The number of such  charges to edge $e$ is bounded by $\frac{D}{\eps \ell(e)}$, and the total number of such inspections is bounded by $\sum_e\frac{D}{\eps \ell(e)}$.
\end{itemize}

We now describe an update operation, when an edge $(u,v)$ of the tree $T$ is deleted, where $u$ is the parent of $v$. As before, we maintain a heap $H$, to which we add all vertices that need to be inspected. We start with $H$ containing just the vertex $v$. In every iteration, we remove the vertex $x$ from the heap $H$ with smallest $\delta(x)$. We then consider, the vertex $y\in H_x$ with minimum $\delta_x(y)+\ell(x,y)$. If this value is no more than $\delta(x)$, then $y$ must be currently attached to the tree $T$, as we will see later. We attach $x$ to $y$.
Otherwise, we increase $\delta(x)$ by $1$. For every neighbor $z$ of $x$ for which $\round_{e=(x,z)}(\delta(x))$ increases, we update the value $\delta_z(x)$ of $x$ in the heap $H_z$ to be $\delta(x)$; if additionally $z$ is a child of $x$ in the tree $T$, then we add $z$ to the heap $H$.


Notice that throughout the algorithm, if a vertex $y$ of $T_v$ is not on the heap $H$ and is not attached to the tree $T$, then it has an ancestor $y'$ in $H$. From Invariants~\ref{inv2: approx father} and \ref{inv2: approx neighbor}, that ancestor has $\delta(y')<\delta(y)$. If $y$ is at the top of the heap $H_x$ and $\delta_x(y)+\ell(x,y)\leq \delta(x)$, then we know that $\delta(y)\leq \delta_x(y)<\delta(x)$, so $\delta(y')<\delta(x)$, and we should have processed $y'$ and not $x$. This concludes the correctness analysis.

Notice that when $\delta(x)$ increases, we need to be able to quickly figure out which edges incident to $x$ to process. This is implemented as follows. Each vertex $x$ has $m$ buckets. The $i$th bucket contains all edges $e$ incident to $x$, for which $\round_e(i)\neq \round_e(i+1)$. So whenever $\delta(x)$ decreases from $i+1$ to $i$, we need to inspect and charge all edges in the $i$th bucket. To initialize, each vertex creates $D$ buckets, which takes $O(nD)$ time. After that, each edge $e$ adds itself to the relevant buckets of its two endpoint: $D/\eps \ell(e)$ buckets per endpoint. So the total time to initialize the buckets is $O(nD)+O(\sum_e\frac{D}{\eps \ell(e)})$. Once the buckets are initialized, we don't need to do anything to maintain them, except inserting/deleting edges. 


\iffalse
One last part is edge insertion, which turns out to be tricky. Suppose we would like to insert an edge $e=(u,v)$, where $\dist_G(s,u)=1000$, $\dist_G(s,v)=1000$, and $\ell(e)=1$. This insertion does not decrease distances. But because we maintain approximate distances from $s$, we may have $\delta(u)=1000$ and $\delta(v)=1000(1+\eps)$. We need to insert a copy $\delta_v(u)$ of $u$ into the heap of $v$, and it is not clear how to do this while maintaining the invariants. In particular, we are not allowed to let $\delta(v)$ decrease, since this will ruin our analysis.

The solution is a bit weird. (Below is my implementation of the idea that was sketched in Bernstein's paper; he refers to other papers for more details; I did not read them).

 Assume that we insert an edge is $e=(u,v)$ and that $\delta(u)\leq \delta(v)$. We add a copy $\delta_u(v)=\delta(v)$ to $H_u$ as usual, and add $e$ to all the relevant buckets of $u$. All invariants continue to hold.
 If $\delta(u)+\ell(u,v)\geq \delta(v)$, then we also add a copy $\delta_v(u)=\delta(u)$ to $H_v$ as usual and add $e$ to all the relevant buckets of $v$. However, if $\delta(u)+\ell(u,v)< \delta(v)$, then we say that $(e,v)$ is a \emph{problematic pair}, and we set $\delta_v(u)=\delta(v)-(u,v)$. We will not update this value $\delta_v(u)$ until $\delta(u)$ becomes greater than $\delta_v(u)$, at which point $(e,v)$ will stop being a problematic pair, and we will add $e$ to the relevant buckets of $v$, and continue as usual. But notice that, while $(e,v)$ remains a problematic pair, $\delta(v)$ will not grow, as $v$ can always connect to the tree through $u$. The intuitive idea for why this work is that the original value $\delta(v)$ was a $(1+\eps)$-approximation on $\dist_G(s,v)$, and, as long as $\delta(u)\leq \delta(v)-\ell(u,v)$, we know that $\dist_G(s,v)\leq \delta(v)$. Since the distances never decrease, we maintain a $(1+\eps)$-approximation.
\fi




\paragraph{Final Running Time Analysis}
Let $E_0$ be the set of edges that were present from the beginning, and $E_1$ the set of edges that were inserted over the course of the algorithm. Then the total running time of the algorithm is: $O(nD)+O(\sum_{e\in E_0\cup E_1}\frac{D}{\eps \ell(e)})$.
